# Supplementary material for: Active Safety Envelopes using Light Curtains with Probabilistic Guarantees
Source: arXiv:2107.04000 source file (2021-07-08)
Supplement: Supplementary file 1 [file 0-instructions.tex]

\subsection{Instructions}

Our supplementary materials contain the follwing:

\begin{enumerate}
    \item Web-based demo of random light curtains.
    \item Appendix: \texttt{appendix.pdf}
    \item Source code: \texttt{code.zip}
\end{enumerate}
\vspace{1em}

The easiest way to access our web-demo is to view the online version hosted on this anonymous website: \href{https://main.d7wss8nx0j99f.amplifyapp.com/}{\underline{\texttt{https://main.d7wss8nx0j99f.amplifyapp.com}}}\\

However, it can also be run locally:
\begin{enumerate}
    \item \texttt{cd} into the folder containing supplementary materials.
    \item Run \texttt{python -m http.server}
    \item Open \texttt{http://127.0.0.1:8000/} in a web browser.
\end{enumerate}
